# Supplementary material for: Prune Wisely, Reconstruct Sharply: Compact 3D Gaussian Splatting via Adaptive Pruning and Difference-of-Gaussian Primitives
Source: arXiv:2602.24136 source file (2026-02-27)
Supplement: Supplementary file 1 [file X_suppl.tex]

\clearpage
\setcounter{page}{1}
\maketitlesupplementary

\setcounter{figure}{0}

\setcounter{table}{0}

\setcounter{section}{0}

\section{Additional Implementation Details}
\label{sec:Implementation}
\subsection{Training Settings}
We basically follow the backbone training settings of 3DGS~\cite{kerbl20233d}. Pruning is activated only after densification has finished. During training, we iteratively compute the average value of $L_1$ over the entire training set, and the Reconstruction-aware Pruning Scheduler uses this statistic to control both the timing and the ratio of pruning. 

For the 3D-DoG primitives, we initialize the scaling factors $[f_x, f_y, f_z]$ to $0.5$ and $f_\alpha$ to $0.1$. Any 3D-DoG primitive with $f_\alpha < 0.01$ is degraded to a standard 3D Gaussian primitive.

\subsection{Baseline Configuration}
In this paper, we avoid methods that rely on additional compact encodings, such as learned codebooks, to reduce the overall model size. This ensures a fair comparison that focuses purely on compressing the number of Gaussian primitives. We therefore select baselines that operate directly on 3D Gaussians.

For each baseline, we use the official implementation released by the respective authors. For MaskGaussian~\cite{liu2025maskgaussian}, we adopt the recommended value $\lambda_{m} = 0.0005$. For GaussianSpa, we use its 3DGS-based implementation~\cite{kerbl20233d} rather than MiniSplatting~\cite{fang2024mini} to ensure a consistent densification strategy. We follow the recommended settings of the published Speedy-Splat implementation~\cite{hanson2025speedy}. In addition, we directly report the evaluation results provided in the PUP-3DGS paper~\cite{hanson2025pup}. 

All baselines are trained with the same dataset splits, image resolution, number of iterations, and optimization settings as the original 3DGS.

\subsection{3D-DoG Rasterization}
\vspace{2mm}\noindent\textbf{Forward:}
Following~\autoref{3DDOG}, we compute the scalings $S_p$ and $\alpha_p$ for the pseudo-Gaussians. We then follow the procedure introduced in~\autoref{3dgsPreliminaries} to obtain the 2D covariance matrices $\Sigma'_i$ and $\Sigma^{p'}_i$. The weights for the primary Gaussians, $\alpha'_i$, are computed as in~\autoref{alphai}, while the pseudo-Gaussian weights $\alpha^{p'}_i$ are obtained as
\begin{equation}
        \alpha^{p'}_i = \alpha_p \exp\!\left(-\tfrac{1}{2} (x - \mu'_i)^{\!T} (\Sigma^{p'}_i)^{-1} (x - \mu'_i)\right).
\end{equation}
Next, we define the effective weight $\beta_i$ as
\begin{equation}
        \beta_i = \alpha'_i - \alpha^{p'}_i,
\end{equation}
and accordingly modify the blending rule to
\begin{equation}
C = \sum_{i} c_i\, \beta_i \prod_{j=1}^{i-1} (1 - \beta_j).
\end{equation}

\noindent\textbf{Backward:}
Recall that in~\autoref{3DDOG}, the 3D-DoG model is defined as the subtraction of a pseudo-Gaussian from a primary Gaussian. To optimize the additional pseudo-Gaussian parameters, we modify the original rasterization implementation. The gradients of the opacity parameter $\alpha$ and the opacity factor $f_\alpha$ are given by
\begin{align}
\frac{\partial L}{\partial \alpha}
&\mathrel = 
\bigl(G - f_p G_p\bigr)\,
\frac{\partial L}{\partial \beta},
\\[4pt]
\frac{\partial L}{\partial f_\alpha}
&\mathrel =
- \alpha \, G_p\,
\frac{\partial L}{\partial \beta},
\end{align}
and the gradients for the scaling factors $[f_x, f_y , f_z]$ are
\begin{align}
\frac{\partial L}{\partial f_x}
&\mathrel = -0.5\,\frac{\partial L}{\partial G_p}\,G_p\,d^2_x,\\[4pt]
\frac{\partial L}{\partial f_y}
&\mathrel = -0.5\,\frac{\partial L}{\partial G_p}\,G_p\,d^2_y,\\[4pt]
\frac{\partial L}{\partial f_z}
&\mathrel = -0.5\,\frac{\partial L}{\partial G_p}\,G_p\,d_x d_y,
\end{align}
where $[d_x, d_y]$ denote the 2D Gaussian pixel offsets, and $\frac{\partial L}{\partial G_p}$ is a temporary variable defined as
\begin{equation}
    \frac{\partial L}{\partial G_p} = -\alpha f_\alpha \frac{\partial L}{\partial \beta}.
\end{equation}

\section{Additional Results}
By adopting the Reconstruction-aware Pruning Scheduler, our method can compress 3DGS models to meet any predefined pruning target. Here, we additionally present results for pruning 50\% and 80\% of primitives. Evaluation results are reported in~\autoref{tab:sup-result}. The results show that our method achieves the best performance on the Deep Blending dataset~\cite{hedman2018deep} and that, across different pruning ratios, the metrics of the compressed models can match those of the 3DGS backbone. Moreover, our method can retain the original performance on Mip-NeRF 360~\cite{barron2022mip} and Tanks and Temples~\cite{knapitsch2017tanks} when pruning 50\% of primitives. Finally, note that our 20\% model can outperform GaussianSpa~\cite{zhang2025gaussianspa} while using less memory.

\begin{table*}[t]
    \centering
    %\footnotesize
    \setlength\tabcolsep{2pt}
    \captionsetup{singlelinecheck=false}
        \caption{Quantitative evaluation of our method using different pruning ratios, computed over three datasets: Mip-NeRF 360, Deep Blending, and Tanks and Temples. $\uparrow$ indicates that larger values are better, while $\downarrow$ indicates the opposite.}
    \resizebox{\textwidth}{!}{
    \begin{tabular} {r | rrrrr | rrrrr | rrrrr}
        \toprule
        \multirow{2}{*}{Method} 
        & \multicolumn{5}{c}{Mip-NeRF 360~\cite{barron2022mip}} & \multicolumn{5}{c}{Deep Blending~\cite{hedman2018deep}} & \multicolumn{5}{c}{Tanks and Temples~\cite{knapitsch2017tanks}} \\
        \cmidrule(l{2pt}r{2pt}){2-6} \cmidrule(l{2pt}r{2pt}){7-11} \cmidrule(l{2pt}r{2pt}){12-16}
        & $\mathrm{ Size}\downarrow$ & PSNR$\uparrow$ & SSIM$\uparrow$ & LPIPS$\downarrow$ &Time$\downarrow$ 
        & $\mathrm{ Size}\downarrow$ & PSNR$\uparrow$ & SSIM$\uparrow$ & LPIPS$\downarrow$ &Time$\downarrow$ 
        & $\mathrm{ Size}\downarrow$ & PSNR$\uparrow$ & SSIM$\uparrow$ & LPIPS$\downarrow$ &Time$\downarrow$ \\
        \midrule
        3DGS~\cite{kerbl20233d}
                          &          645.2 &          27.47 &          0.826 &          0.201 &          17m1s 
                          &          592.7 &          29.75 &          0.904 &          0.244 &          13m51s 
                          &          381.0 &          23.77 &          0.847 &          0.177 &          17m50s \\

        \midrule
         Ours-50\%
                            &          328.3 &         27.51 &          0.815 &         0.217 &          15m42s 
                            &          300.5 &         29.89 &      0.905         &  0.242            &    12m3s    &  192.2  & 23.81
                            &       0.851        &       0.171     &     11m43s              \\
         Ours-20\%
                          &          131.5 &         27.47  &          0.809 &          0.241&          14m10s
                          &          120.2 &           29.87 &         0.905 &        0.241 &          10m41s  
                          &            76.8       &  23.71
                          &       0.843       &   0.195  &  8m42s \\
        Ours-10\%
                          &          65.3 &          27.16 &          0.789 &          0.285 &          13m48s
                          &          59.9 &          29.87 &          0.904 &          0.254 &           10m19s 
                          &          38.4 &          23.79 &          0.823 &         0.229 &           8m9s \\
        \bottomrule
    \end{tabular}
    }
    \label{tab:sup-result}
\end{table*}
